# Supplementary material for: On the possibility of differential-algebraic elimination of the spinor field from the Maxwell--Dirac electrodynamics
Source: arXiv:2602.15907 ancillary file (2026-06-08)
Supplement: Supplementary file 1 [file nplow4.pdf]

```
restart;
libname := "c:\\qm\\dt\\dt", libname;
"c:\\qm\\dt\\dt", "C:\\Program Files\\Maple 2016\\lib" (1)
```

```
with(DifferentialThomas);
[CallJets, CheckResult, CheckResults, ClearRememberData, ComparePolyInfo, (2)
```

```
ComplementOfDecomposition, ComputeRanking, ComputeWithDiffalg, Diff2JetList,
DifferentialSystemCartanCharacters, DifferentialSystemDimensionPolynomial,
DifferentialSystemDimensionPolynomialCanonicalBase, DifferentialSystemEquations,
DifferentialSystemFactorModuleBasis, DifferentialSystemHilbertPolynomial,
DifferentialSystemHilbertPolynomialCanonicalBase, DifferentialSystemHilbertSeries,
DifferentialSystemInequations, DifferentialSystemLinearCombination,
DifferentialSystemNormalForm, DifferentialSystemPrincipalDerivatives,
DifferentialSystemReduce, DifferentialSystemStrength, DifferentialThomasDecomposition,
DifferentialThomasNewOptions, DifferentialThomasOptions, InconsistentPolynom, Initial,
IntersectDecompositions, JetList2Diff, LastCommonSystemInHistory, Leader,
LeadingDerivation, LeadingFunction, MaxOrder, MyPDSolve, OrderofLeader,
PartialDerivative, PowerSeriesSolution, PrettyPrintDifferentialSystem,
PrintDifferentialSystem, PrintDifferentialSystemJanetTrees,
PrintDifferentialSystemJanetTreesCombinatorics, PrintHistory, PrintRanking, Rank,
RemoveSuperflousInequations, ReturnInDoNextStepAndSetOrders, Separant,
SimplifyInequationsInDifferentialSystem, StandardForm, SystemTime, Walk]
```

```
st42 := time( ) : ivar := [x0, x1, x2, x3];
#x0 - time, x1,x2,x3 - coordinates
[x0, x1, x2, x3] (3)
```

```
dvar := [a0, ps4i, ps4r, ps3i, ps3r, ps2i, ps2r, ps1r, a3, a2, a1, e2];
#a0,a1,a2,a3 - components of the electromagnetic 4-potential, first component of the Dirac spinor ps1r
#is real (gauge condition), the other components of the Dirac spinor are ps2r + I·ps2i and so on, e3 is
#the square of the elementary charge
[a0, ps4i, ps4r, ps3i, ps3r, ps2i, ps2r, ps1r, a3, a2, a1, e2] (4)
```

```
nops(ivar);
4 (5)
```

```
nops(dvar);
12 (6)
```

```
eq1 := e2[1, 0, 0, 0];
e21, 0, 0, 0 (7)
```

```
eq2 := e2[0, 1, 0, 0];
e20, 1, 0, 0 (8)
```

```
eq3 := e2[0, 0, 1, 0];
e20, 0, 1, 0 (9)
```

```
eq4 := e2[0, 0, 0, 1];
e20, 0, 0, 1 (10)
```

```
d1 := (a0[0, 0, 0, 0] + a3[0, 0, 0, 0]) · (ps3r[0, 0, 0, 0] + I·ps3i[0, 0, 0, 0]) + (a1[0, 0, 0, 0] - I
```

$$\cdot a2[0, 0, 0, 0]) \cdot (ps4r[0, 0, 0, 0] + I \cdot ps4i[0, 0, 0, 0]) + I \cdot ((ps3r[0, 0, 0, 1] + I \cdot ps3i[0, 0, 0, 1]) - I \cdot (ps4r[0, 0, 1, 0] + I \cdot ps4i[0, 0, 1, 0]) + (ps4r[0, 1, 0, 0] + I \cdot ps4i[0, 1, 0, 0]) - (ps3r[1, 0, 0, 0] + I \cdot ps3i[1, 0, 0, 0])) - (ps1r[0, 0, 0, 0]);$$

#d1,d2,d3,d4 are the components of the Dirac equation, d1c,d2c,d3c,d4c - their complex conjugates,  
#chiral representation of the gamma-matrices is used, metric tensor signature is +---

$$(a0_{0,0,0,0} + a3_{0,0,0,0}) (ps3r_{0,0,0,0} + I ps3i_{0,0,0,0}) + (a1_{0,0,0,0} - I a2_{0,0,0,0}) (ps4r_{0,0,0,0} + I ps4i_{0,0,0,0}) + I (ps3r_{0,0,0,1} + I ps3i_{0,0,0,1} - I (ps4r_{0,0,1,0} + I ps4i_{0,0,1,0}) + ps4r_{0,1,0,0} + I ps4i_{0,1,0,0} - ps3r_{1,0,0,0} - I ps3i_{1,0,0,0}) - ps1r_{0,0,0,0} \quad (11)$$

$$d1c := (a0[0, 0, 0, 0] + a3[0, 0, 0, 0]) \cdot (ps3r[0, 0, 0, 0] - I \cdot ps3i[0, 0, 0, 0]) + (a1[0, 0, 0, 0] + I \cdot a2[0, 0, 0, 0]) \cdot (ps4r[0, 0, 0, 0] - I \cdot ps4i[0, 0, 0, 0]) - I \cdot ((ps3r[0, 0, 0, 1] - I \cdot ps3i[0, 0, 0, 1]) + I \cdot (ps4r[0, 0, 1, 0] - I \cdot ps4i[0, 0, 1, 0]) + (ps4r[0, 1, 0, 0] - I \cdot ps4i[0, 1, 0, 0]) - (ps3r[1, 0, 0, 0] - I \cdot ps3i[1, 0, 0, 0])) - (ps1r[0, 0, 0, 0]);$$

$$(a0_{0,0,0,0} + a3_{0,0,0,0}) (ps3r_{0,0,0,0} - I ps3i_{0,0,0,0}) + (a1_{0,0,0,0} + I a2_{0,0,0,0}) (ps4r_{0,0,0,0} - I ps4i_{0,0,0,0}) - I (ps3r_{0,0,0,1} - I ps3i_{0,0,0,1} + I (ps4r_{0,0,1,0} - I ps4i_{0,0,1,0}) + ps4r_{0,1,0,0} - I ps4i_{0,1,0,0} - ps3r_{1,0,0,0} + I ps3i_{1,0,0,0}) - ps1r_{0,0,0,0} \quad (12)$$

$$eq5 := \text{simplify}\left(\frac{(d1 + d1c)}{2}\right);$$

$$(a0_{0,0,0,0} + a3_{0,0,0,0}) ps3r_{0,0,0,0} + a1_{0,0,0,0} ps4r_{0,0,0,0} + a2_{0,0,0,0} ps4i_{0,0,0,0} + ps3i_{1,0,0,0} - ps4i_{0,1,0,0} + ps4r_{0,0,1,0} - ps1r_{0,0,0,0} - ps3i_{0,0,0,1} \quad (13)$$

$$eq6 := \text{simplify}\left(\frac{(d1 - d1c)}{2 \cdot I}\right);$$

$$(a0_{0,0,0,0} + a3_{0,0,0,0}) ps3i_{0,0,0,0} + a1_{0,0,0,0} ps4i_{0,0,0,0} - a2_{0,0,0,0} ps4r_{0,0,0,0} + ps4i_{0,0,1,0} + ps4r_{0,1,0,0} + ps3r_{0,0,0,1} - ps3r_{1,0,0,0} \quad (14)$$

$$d2 := (a1[0, 0, 0, 0] + I \cdot a2[0, 0, 0, 0]) \cdot (ps3r[0, 0, 0, 0] + I \cdot ps3i[0, 0, 0, 0]) + (a0[0, 0, 0, 0] - a3[0, 0, 0, 0]) \cdot (ps4r[0, 0, 0, 0] + I \cdot ps4i[0, 0, 0, 0]) - I \cdot ((ps4r[0, 0, 0, 1] + I \cdot ps4i[0, 0, 0, 1]) - I \cdot (ps3r[0, 0, 1, 0] + I \cdot ps3i[0, 0, 1, 0]) - (ps3r[0, 1, 0, 0] + I \cdot ps3i[0, 1, 0, 0]) + (ps4r[1, 0, 0, 0] + I \cdot ps4i[1, 0, 0, 0])) - (ps2r[0, 0, 0, 0] + I \cdot ps2i[0, 0, 0, 0]);$$

$$(a1_{0,0,0,0} + I a2_{0,0,0,0}) (ps3r_{0,0,0,0} + I ps3i_{0,0,0,0}) + (a0_{0,0,0,0} - a3_{0,0,0,0}) (ps4r_{0,0,0,0} + I ps4i_{0,0,0,0}) - I (ps4r_{0,0,0,1} + I ps4i_{0,0,0,1} - I (ps3r_{0,0,1,0} + I ps3i_{0,0,1,0}) - ps3r_{0,1,0,0} - I ps3i_{0,1,0,0} + ps4r_{1,0,0,0} + I ps4i_{1,0,0,0}) - ps2r_{0,0,0,0} - I ps2i_{0,0,0,0} \quad (15)$$

$$d2c := (a1[0, 0, 0, 0] - I \cdot a2[0, 0, 0, 0]) \cdot (ps3r[0, 0, 0, 0] - I \cdot ps3i[0, 0, 0, 0]) + (a0[0, 0, 0, 0] - a3[0, 0, 0, 0]) \cdot (ps4r[0, 0, 0, 0] - I \cdot ps4i[0, 0, 0, 0]) + I \cdot ((ps4r[0, 0, 0, 1] - I \cdot ps4i[0, 0, 0, 1]) + I \cdot (ps3r[0, 0, 1, 0] - I \cdot ps3i[0, 0, 1, 0]) - (ps3r[0, 1, 0, 0] - I \cdot ps3i[0, 1, 0, 0]) + (ps4r[1, 0, 0, 0] - I \cdot ps4i[1, 0, 0, 0])) - (ps2r[0, 0, 0, 0] - I \cdot ps2i[0, 0, 0, 0]);$$

$$(a1_{0,0,0,0} - I a2_{0,0,0,0}) (ps3r_{0,0,0,0} - I ps3i_{0,0,0,0}) + (a0_{0,0,0,0} - a3_{0,0,0,0}) (ps4r_{0,0,0,0} - I ps4i_{0,0,0,0}) + I (ps4r_{0,0,0,1} - I ps4i_{0,0,0,1} + I (ps3r_{0,0,1,0} - I ps3i_{0,0,1,0}) - ps3r_{0,1,0,0} + I ps3i_{0,1,0,0} + ps4r_{1,0,0,0} - I ps4i_{1,0,0,0}) - ps2r_{0,0,0,0} + I ps2i_{0,0,0,0} \quad (16)$$

$$eq7 := \text{simplify}\left(\frac{(d2 + d2c)}{2}\right);$$

$$(a0_{0,0,0,0} - a3_{0,0,0,0}) ps4r_{0,0,0,0} + a1_{0,0,0,0} ps3r_{0,0,0,0} - a2_{0,0,0,0} ps3i_{0,0,0,0} - ps3r_{0,0,1,0} + ps4i_{0,0,0,1} + ps4i_{1,0,0,0} - ps2r_{0,0,0,0} - ps3i_{0,1,0,0} \quad (17)$$

$$eq8 := simplify\left(\frac{(d2 - d2c)}{2 \cdot I}\right);$$

$$(a0_{0,0,0,0} - a3_{0,0,0,0}) ps4i_{0,0,0,0} + a1_{0,0,0,0} ps3i_{0,0,0,0} + a2_{0,0,0,0} ps3r_{0,0,0,0} + ps3r_{0,1,0,0} \quad (18)$$

$$- ps4r_{0,0,0,1} - ps4r_{1,0,0,0} - ps2i_{0,0,0,0} - ps3i_{0,0,1,0}$$

$$d3 := (a0[0,0,0,0] - a3[0,0,0,0]) \cdot (ps1r[0,0,0,0]) - (a1[0,0,0,0] - I \cdot a2[0,0,0,0]) \cdot (ps2r[0,0,0,0] + I \cdot ps2i[0,0,0,0]) - I \cdot ((ps1r[0,0,0,1]) - I \cdot (ps2r[0,0,1,0] + I \cdot ps2i[0,0,1,0]) + (ps2r[0,1,0,0] + I \cdot ps2i[0,1,0,0]) + (ps1r[1,0,0,0])) - (ps3r[0,0,0,0] + I \cdot ps3i[0,0,0,0]);$$

$$(a0_{0,0,0,0} - a3_{0,0,0,0}) ps1r_{0,0,0,0} - (a1_{0,0,0,0} - I a2_{0,0,0,0}) (ps2r_{0,0,0,0} + I ps2i_{0,0,0,0}) \quad (19)$$

$$- I (ps1r_{0,0,0,1} - I (ps2r_{0,0,1,0} + I ps2i_{0,0,1,0}) + ps2r_{0,1,0,0} + I ps2i_{0,1,0,0} + ps1r_{1,0,0,0}) - ps3r_{0,0,0,0} - I ps3i_{0,0,0,0}$$

$$d3c := (a0[0,0,0,0] - a3[0,0,0,0]) \cdot (ps1r[0,0,0,0]) - (a1[0,0,0,0] + I \cdot a2[0,0,0,0]) \cdot (ps2r[0,0,0,0] - I \cdot ps2i[0,0,0,0]) + I \cdot ((ps1r[0,0,0,1]) + I \cdot (ps2r[0,0,1,0] - I \cdot ps2i[0,0,1,0]) + (ps2r[0,1,0,0] - I \cdot ps2i[0,1,0,0]) + (ps1r[1,0,0,0])) - (ps3r[0,0,0,0] - I \cdot ps3i[0,0,0,0]);$$

$$(a0_{0,0,0,0} - a3_{0,0,0,0}) ps1r_{0,0,0,0} - (a1_{0,0,0,0} + I a2_{0,0,0,0}) (ps2r_{0,0,0,0} - I ps2i_{0,0,0,0}) \quad (20)$$

$$+ I (ps1r_{0,0,0,1} + I (ps2r_{0,0,1,0} - I ps2i_{0,0,1,0}) + ps2r_{0,1,0,0} - I ps2i_{0,1,0,0} + ps1r_{1,0,0,0}) - ps3r_{0,0,0,0} + I ps3i_{0,0,0,0}$$

$$eq9 := simplify\left(\frac{(d3 + d3c)}{2}\right);$$

$$(a0_{0,0,0,0} - a3_{0,0,0,0}) ps1r_{0,0,0,0} - a1_{0,0,0,0} ps2r_{0,0,0,0} - a2_{0,0,0,0} ps2i_{0,0,0,0} - ps2r_{0,0,1,0} \quad (21)$$

$$- ps3r_{0,0,0,0} + ps2i_{0,1,0,0}$$

$$eq10 := simplify\left(\frac{(d3 - d3c)}{2 \cdot I}\right);$$

$$- a1_{0,0,0,0} ps2i_{0,0,0,0} + a2_{0,0,0,0} ps2r_{0,0,0,0} - ps1r_{0,0,0,1} - ps1r_{1,0,0,0} - ps2i_{0,0,1,0} \quad (22)$$

$$- ps2r_{0,1,0,0} - ps3i_{0,0,0,0}$$

$$d4 := - (a1[0,0,0,0] + I \cdot a2[0,0,0,0]) \cdot (ps1r[0,0,0,0]) + (a0[0,0,0,0] + a3[0,0,0,0]) \cdot (ps2r[0,0,0,0] + I \cdot ps2i[0,0,0,0]) + I \cdot (ps2r[0,0,0,1] + I \cdot ps2i[0,0,0,1]) + (ps1r[0,0,1,0]) - I \cdot (ps1r[0,1,0,0]) - I \cdot (ps2r[1,0,0,0] + I \cdot ps2i[1,0,0,0]) - (ps4r[0,0,0,0] + I \cdot ps4i[0,0,0,0]);$$

$$- (a1_{0,0,0,0} + I a2_{0,0,0,0}) ps1r_{0,0,0,0} + (a0_{0,0,0,0} + a3_{0,0,0,0}) (ps2r_{0,0,0,0} + I ps2i_{0,0,0,0}) \quad (23)$$

$$+ I (ps2r_{0,0,0,1} + I ps2i_{0,0,0,1}) + ps1r_{0,0,1,0} - I ps1r_{0,1,0,0} - I (ps2r_{1,0,0,0} + I ps2i_{1,0,0,0}) - ps4r_{0,0,0,0} - I ps4i_{0,0,0,0}$$

$$d4c := - (a1[0,0,0,0] - I \cdot a2[0,0,0,0]) \cdot (ps1r[0,0,0,0]) + (a0[0,0,0,0] + a3[0,0,0,0]) \cdot (ps2r[0,0,0,0] - I \cdot ps2i[0,0,0,0]) - I \cdot (ps2r[0,0,0,1] - I \cdot ps2i[0,0,0,1]) + (ps1r[0,0,1,0]) + I \cdot (ps1r[0,1,0,0]) + I \cdot (ps2r[1,0,0,0] - I \cdot ps2i[1,0,0,0]) - (ps4r[0,0,0,0] - I \cdot ps4i[0,0,0,0]);$$

$$- (a1_{0,0,0,0} - I a2_{0,0,0,0}) ps1r_{0,0,0,0} + (a0_{0,0,0,0} + a3_{0,0,0,0}) (ps2r_{0,0,0,0} - I ps2i_{0,0,0,0}) \quad (24)$$

$$- I (ps2r_{0,0,0,1} - I ps2i_{0,0,0,1}) + ps1r_{0,0,1,0} + I ps1r_{0,1,0,0} + I (ps2r_{1,0,0,0} - I ps2i_{1,0,0,0}) - ps4r_{0,0,0,0} + I ps4i_{0,0,0,0}$$

$$eq11 := simplify\left(\frac{(d4 + d4c)}{2}\right);$$

$$(a0_{0,0,0,0} + a3_{0,0,0,0})ps2r_{0,0,0,0} - a1_{0,0,0,0}ps1r_{0,0,0,0} - ps4r_{0,0,0,0} + ps1r_{0,0,1,0} - ps2i_{0,0,0,1} + ps2i_{1,0,0,0} \quad (25)$$

$$eq12 := simplify\left(\frac{(d4 - d4c)}{2 \cdot I}\right);$$

$$(a0_{0,0,0,0} + a3_{0,0,0,0})ps2i_{0,0,0,0} - a2_{0,0,0,0}ps1r_{0,0,0,0} - ps4i_{0,0,0,0} - ps1r_{0,0,1,0} + ps2r_{0,0,0,1} - ps2r_{1,0,0,0} \quad (26)$$

$$gs1 := Matrix(2, 2, [[0, 1], [1, 0]]);$$

$$\begin{bmatrix} 0 & 1 \\ 1 & 0 \end{bmatrix} \quad (27)$$

$$gs2 := Matrix(2, 2, [[0, -I], [I, 0]]);$$

$$\begin{bmatrix} 0 & -I \\ I & 0 \end{bmatrix} \quad (28)$$

$$gs3 := Matrix(2, 2, [[1, 0], [0, -1]]);$$

$$\begin{bmatrix} 1 & 0 \\ 0 & -1 \end{bmatrix} \quad (29)$$

$$psisqup := Matrix(2, 1, [[(ps1r[0, 0, 0, 0])], [(ps2r[0, 0, 0, 0] + I \cdot ps2i[0, 0, 0, 0])]]);$$

$$\begin{bmatrix} ps1r_{0,0,0,0} \\ ps2r_{0,0,0,0} + Ips2i_{0,0,0,0} \end{bmatrix} \quad (30)$$

$$psisqupd := Matrix(1, 2, [(ps1r[0, 0, 0, 0]), (ps2r[0, 0, 0, 0] - I \cdot ps2i[0, 0, 0, 0])]);$$

$$\begin{bmatrix} ps1r_{0,0,0,0} & ps2r_{0,0,0,0} - Ips2i_{0,0,0,0} \end{bmatrix} \quad (31)$$

$$psisqdown := Matrix(2, 1, [[(ps3r[0, 0, 0, 0] + I \cdot ps3i[0, 0, 0, 0])], [(ps4r[0, 0, 0, 0] + I \cdot ps4i[0, 0, 0, 0])]]);$$

$$\begin{bmatrix} ps3r_{0,0,0,0} + Ips3i_{0,0,0,0} \\ ps4r_{0,0,0,0} + Ips4i_{0,0,0,0} \end{bmatrix} \quad (32)$$

$$psisqdownnd := Matrix(1, 2, [(ps3r[0, 0, 0, 0] - I \cdot ps3i[0, 0, 0, 0]), (ps4r[0, 0, 0, 0] - I \cdot ps4i[0, 0, 0, 0])]);$$

$$\begin{bmatrix} ps3r_{0,0,0,0} - Ips3i_{0,0,0,0} & ps4r_{0,0,0,0} - Ips4i_{0,0,0,0} \end{bmatrix} \quad (33)$$

$$jj0 := simplify((ps1r[0, 0, 0, 0]) \cdot (ps1r[0, 0, 0, 0]) + (ps2r[0, 0, 0, 0] + I \cdot ps2i[0, 0, 0, 0]) \cdot (ps2r[0, 0, 0, 0] - I \cdot ps2i[0, 0, 0, 0]) + (ps3r[0, 0, 0, 0] + I \cdot ps3i[0, 0, 0, 0]) \cdot (ps3r[0, 0, 0, 0] - I \cdot ps3i[0, 0, 0, 0]) + (ps4r[0, 0, 0, 0] + I \cdot ps4i[0, 0, 0, 0]) \cdot (ps4r[0, 0, 0, 0] - I \cdot ps4i[0, 0, 0, 0]));$$

#jj0,jj1,jj2,jj3 —components of the Dirac current (up to a constant factor)

$$ps1r_{0,0,0,0}^2 + ps2i_{0,0,0,0}^2 + ps2r_{0,0,0,0}^2 + ps3i_{0,0,0,0}^2 + ps3r_{0,0,0,0}^2 + ps4i_{0,0,0,0}^2 + ps4r_{0,0,0,0}^2 \quad (34)$$

with(LinearAlgebra) :

$$jj1 := simplify((Multiply(psisqupd, Multiply(gs1, psisqup)) - Multiply(psisqdownnd, Multiply(gs1, psisqdown)))(1, 1));$$

$$2 ps1r_{0,0,0,0} ps2r_{0,0,0,0} - 2 ps3i_{0,0,0,0} ps4i_{0,0,0,0} - 2 ps3r_{0,0,0,0} ps4r_{0,0,0,0} \quad (35)$$

$jj2 := \text{simplify}((\text{Multiply}(\text{psisqupd}, \text{Multiply}(\text{gs2}, \text{psisqup})) - \text{Multiply}(\text{psisqdown}, \text{Multiply}(\text{gs2}, \text{psisqdown}))) (1, 1));$

$$2 ps1r_{0,0,0,0} ps2i_{0,0,0,0} + 2 ps3i_{0,0,0,0} ps4r_{0,0,0,0} - 2 ps3r_{0,0,0,0} ps4i_{0,0,0,0} \quad (36)$$

$jj3 := \text{simplify}((\text{Multiply}(\text{psisqupd}, \text{Multiply}(\text{gs3}, \text{psisqup})) - \text{Multiply}(\text{psisqdown}, \text{Multiply}(\text{gs3}, \text{psisqdown}))) (1, 1));$

$$ps1r_{0,0,0,0}^2 - ps2i_{0,0,0,0}^2 - ps2r_{0,0,0,0}^2 - ps3i_{0,0,0,0}^2 - ps3r_{0,0,0,0}^2 + ps4i_{0,0,0,0}^2 + ps4r_{0,0,0,0}^2 \quad (37)$$

$eq13 := a0[2, 0, 0, 0] - a0[0, 2, 0, 0] - a0[0, 0, 2, 0] - a0[0, 0, 0, 2] - a0[2, 0, 0, 0] - a1[1, 1, 0, 0] - a2[1, 0, 1, 0] - a3[1, 0, 0, 1] - e2 \cdot jj0;$

#eq13-16 - Maxwell equations

$$-a0_{0,2,0,0} - a0_{0,0,2,0} - a0_{0,0,0,2} - a1_{1,1,0,0} - a2_{1,0,1,0} - a3_{1,0,0,1} - e2 (ps1r_{0,0,0,0}^2 + ps2i_{0,0,0,0}^2 + ps2r_{0,0,0,0}^2 + ps3i_{0,0,0,0}^2 + ps3r_{0,0,0,0}^2 + ps4i_{0,0,0,0}^2 + ps4r_{0,0,0,0}^2) \quad (38)$$

$eq14 := -(a1[2, 0, 0, 0] - a1[0, 2, 0, 0] - a1[0, 0, 2, 0] - a1[0, 0, 0, 2]) - a0[1, 1, 0, 0] - a1[0, 2, 0, 0] - a2[0, 1, 1, 0] - a3[0, 1, 0, 1] + e2 \cdot jj1;$

$$-a1_{2,0,0,0} + a1_{0,0,2,0} + a1_{0,0,0,2} - a0_{1,1,0,0} - a2_{0,1,1,0} - a3_{0,1,0,1} + e2 (2 ps1r_{0,0,0,0} ps2r_{0,0,0,0} - 2 ps3i_{0,0,0,0} ps4i_{0,0,0,0} - 2 ps3r_{0,0,0,0} ps4r_{0,0,0,0}) \quad (39)$$

$eq15 := -(a2[2, 0, 0, 0] - a2[0, 2, 0, 0] - a2[0, 0, 2, 0] - a2[0, 0, 0, 2]) - a0[1, 0, 1, 0] - a1[0, 1, 1, 0] - a2[0, 0, 2, 0] - a3[0, 0, 1, 1] + e2 \cdot jj2;$

$$-a2_{2,0,0,0} + a2_{0,2,0,0} + a2_{0,0,2,0} - a0_{1,0,1,0} - a1_{0,1,1,0} - a3_{0,0,1,1} + e2 (2 ps1r_{0,0,0,0} ps2i_{0,0,0,0} + 2 ps3i_{0,0,0,0} ps4r_{0,0,0,0} - 2 ps3r_{0,0,0,0} ps4i_{0,0,0,0}) \quad (40)$$

$eq16 := -(a3[2, 0, 0, 0] - a3[0, 2, 0, 0] - a3[0, 0, 2, 0] - a3[0, 0, 0, 2]) - a0[1, 0, 0, 1] - a1[0, 1, 0, 1] - a2[0, 0, 1, 1] - a3[0, 0, 0, 2] + e2 \cdot jj3;$

$$-a3_{2,0,0,0} + a3_{0,2,0,0} + a3_{0,0,2,0} - a0_{1,0,0,1} - a1_{0,1,0,1} - a2_{0,0,1,1} + e2 (ps1r_{0,0,0,0}^2 - ps2i_{0,0,0,0}^2 - ps2r_{0,0,0,0}^2 - ps3i_{0,0,0,0}^2 - ps3r_{0,0,0,0}^2 + ps4i_{0,0,0,0}^2 + ps4r_{0,0,0,0}^2) \quad (41)$$

$L0 := [eq1, eq2, eq3, eq4, eq5, eq6, eq7, eq8, eq9, eq10, eq11, eq12, eq13, eq14, eq15, eq16];$

$L1 := L0;$

$$\begin{aligned} & \text{dvarnp} := [a0, ps4i, ps4r, ps3i, ps3r, ps2i, ps2r, a3, a2, a1, ps1r, e2]; \\ & \text{dvarnp} := [a0, ps4i, ps4r, ps3i, ps3r, ps2i, ps2r, a3, a2, a1, ps1r, e2] \end{aligned} \quad (42)$$

$\text{ComputeRanking}(\text{ivar}, \text{dvarnp}, \text{"DegRevLex"});$

$\text{DifferentialThomasOptions}(\text{"SelectionStrategy"}, \text{"SmallestElement"});$

$\text{DifferentialThomasOptions}(\text{"CompareStrategy"}, \text{"ByEquationThenRanking"});$

$\text{DifferentialThomasOptions}(\text{"SortFactors"}, \text{"Generic"});$

$\text{DifferentialThomasOptions}(\text{"TailReduction"}, \text{true});$

$\text{DifferentialThomasOptions}(\text{"ReduceQListInSystem"}, \text{"Inequations"});$

$\text{DifferentialThomasOptions}(\text{"Factor"}, \text{true});$

$\text{DifferentialThomasOptions}(\text{"FactorStrong"}, \text{false});$

$\text{DifferentialThomasOptions}(\text{"FinalTailReduction"}, \text{true});$

$\text{DifferentialThomasOptions}(\text{"ResultantStrategy"}, \text{"PRS"});$

$\text{DifferentialThomasOptions}(\text{"ReductionOld"}, \text{false});$

$\text{DifferentialThomasOptions}(\text{"MaxSizeMultiplicator"}, \text{infinity});$

$\text{DifferentialThomasOptions}(\text{"ReductionFactor"}, \text{false});$

$\text{DifferentialThomasOptions}(\text{"TailReductionIntermediate"}, \text{false});$

$\text{DifferentialThomasOptions}(\text{"MaxSizeMultiplicatorIntermediate"}, \text{infinity});$

```
DifferentialThomasOptions("OftenRemoveContent", true) :
DifferentialThomasOptions("FactorInequations", true) :
DifferentialThomasOptions("InequationsNotCoprime", false) :
DifferentialThomasOptions("InequationsNotSquarefree", false) :
LI[16];
```

$$-a^3_{2,0,0,0} + a^3_{0,2,0,0} + a^3_{0,0,2,0} - a^0_{1,0,0,1} - a^1_{0,1,0,1} - a^2_{0,0,1,1} + e^2 \left( ps1r^2_{0,0,0,0} - ps2i^2_{0,0,0,0} - ps2r^2_{0,0,0,0} - ps3i^2_{0,0,0,0} - ps3r^2_{0,0,0,0} + ps4i^2_{0,0,0,0} + ps4r^2_{0,0,0,0} \right) \quad (43)$$

```
[> resnp := DifferentialThomasDecomposition(LI, [e2[0,0,0,0], ps1r[0,0,0,0]]);
      resnp := [DifferentialSystem]
[> #PrintDifferentialSystem(resnp[1]) : \quad (44)
```

```
> dvarnp2 := [a0, a1, ps4i, ps4r, ps3i, ps3r, ps2i, ps2r, ps1r, a3, a2, e2];
      dvarnp2 := [a0, a1, ps4i, ps4r, ps3i, ps3r, ps2i, ps2r, ps1r, a3, a2, e2] \quad (1.1)
```

```
> MonomialList := ee → 'if'(type(ee, '+'), convert(ee, list), [ee]);
      MonomialList := ee → if(type(ee, '+'), convert(ee, list), [ee]) \quad (1.2)
```

```
> ktay := 6; #the number of prolongations of each equation
      ktay := 6 \quad (1.3)
```

```
> psa := array(1..11, 0..ktay+2, 0..ktay+2, 0..ktay+2, 0..ktay+2) :
```

```
> renpr := proc( a73 )
      #description "rename, e.g., ps4i[0,0,0,0] as psa[1,0,0,0]":
      if op(0, a73) = ps4i then ii00 := 1 :
      elif op(0, a73) = ps4r then ii00 := 2 :
      elif op(0, a73) = ps3i then ii00 := 3 :
      elif op(0, a73) = ps3r then ii00 := 4 :
      elif op(0, a73) = ps2i then ii00 := 5 :
      elif op(0, a73) = ps2r then ii00 := 6 :
      elif op(0, a73) = ps1r then ii00 := 7 :
      elif op(0, a73) = a0 then ii00 := 8 :
      elif op(0, a73) = a3 then ii00 := 9 :
      elif op(0, a73) = a2 then ii00 := 10 :
      elif op(0, a73) = a1 then ii00 := 11 :
      end if:
      psa[ii00, op(1, a73), op(2, a73), op(3, a73), op(4, a73)] :
```

```
end proc:
Warning, `ii00` is implicitly declared local to procedure
`renpr`
```

```
> reneq := proc( a74 )
      #description "in an equation, rename indets, e.g., ps4i[0,0,0,0] as psa[1,0,0,0]":
      a74int := eval( a74, e2[0,0,0,0] = 221/2410 ) :
      a74int := eval( a74int, e2 = 221/2410 ) :
      eval( evalindets(a74int, indets(a74int), vvv → renpr(vvv) ) ) :
```

```
end proc:
Warning, `a74int` is implicitly declared local to procedure
```

`renew`

```
> combi := Array:#to store combination numbers for differentiation of products
> for nn from 0 to ktay + 4 do:
  for mm from 0 to nn do:
    combi[nn, mm] := combinat:numbcomb(nn, mm) :
  end do:
end do:
> mondifcor := proc( a75, jj0, jj1, jj2, jj3 )

  #description "differentiation of a monomial (including no more than 2 factors psa[]) jj0,
  jj1, jj2, jj3 times with respect to x0, x1, x2, x3, respectively":
  indmon := indets(a75) :
  nuind := numelems(indmon) :
  if nuind = 0 then
    if jj0 + jj1 + jj2 + jj3 = 0 then return a75 :
    else return 0 :
    end if:
  elif nuind = 1 then fact1 := op(1, indmon) : deg1 := degree(a75, fact1) :
    if deg1 = 1 then coef1 := coeff(a75, fact1) : return coef1·op(0, fact1)[op(1, fact1),
    op(2, fact1) + jj0, op(3, fact1) + jj1, op(4, fact1) + jj2, op(5, fact1) + jj3] :
    else coef1 := coeff(a75, fact1, 2) : fact2 := fact1 :
    end if:
  else fact1 := op(1, indmon) : fact2 := op(2, indmon) : coef1 := coeff(coeff(a75, fact1),
  fact2) :
  end if:
  #print( fact1, fact2, coef1) :
  op10 := op(0, fact1) :
  #print(op10) :
  op20 := op(0, fact2) :
  op1 := [op(fact1)] :
  op2 := [op(fact2)] :
  #print(op10, op20, op1, op2) :
  sum7 := 0 :
  for jj0cur from 0 to jj0 do:
    for jj1cur from 0 to jj1 do:
      for jj2cur from 0 to jj2 do:
        for jj3cur from 0 to jj3 do:
          sum7 := sum7 + combi[jj0, jj0cur]·combi[jj1, jj1cur]·combi[jj2, jj2cur]
          ·combi[jj3, jj3cur]·op10[op1[1], op1[2] + jj0cur, op1[3] + jj1cur, op1[4] + jj2cur,
          op1[5] + jj3cur]·op20[op2[1], op2[2] + jj0 - jj0cur, op2[3] + jj1 - jj1cur, op2[4]
          + jj2 - jj2cur, op2[5] + jj3 - jj3cur] :
          #sum7:=sum7+combi(jj0, jj0cur)·combi(jj1, jj1cur)·combi(jj2, jj2cur)
          ·combi(jj3, jj3cur)·op(0, fact1)[[op(fact1)][1], [op(fact1)][2] + jj0cur,
          [op(fact1)][3] + jj1cur, [op(fact1)][4] + jj2cur, [op(fact1)][5] + jj3cur]
          ·[op(fact2)][op2[1], [op(fact2)][2] + jj0 - jj0cur, [op(fact2)][3] + jj1 - jj1cur,
          [op(fact2)][4] + jj2 - jj2cur, [op(fact2)][5] + jj3 - jj3cur] :
        end do:
      end do:
    end do:
  end do:
  coef1·sum7 :
end proc:
```

Warning, `indmon` is implicitly declared local to procedure  
`mondifcor`  
Warning, `nuind` is implicitly declared local to procedure  
`mondifcor`  
Warning, `fact1` is implicitly declared local to procedure  
`mondifcor`  
Warning, `deg1` is implicitly declared local to procedure  
`mondifcor`  
Warning, `coef1` is implicitly declared local to procedure  
`mondifcor`  
Warning, `fact2` is implicitly declared local to procedure  
`mondifcor`  
Warning, `op10` is implicitly declared local to procedure  
`mondifcor`  
Warning, `op20` is implicitly declared local to procedure  
`mondifcor`  
Warning, `op1` is implicitly declared local to procedure  
`mondifcor`  
Warning, `op2` is implicitly declared local to procedure  
`mondifcor`  
Warning, `sum7` is implicitly declared local to procedure  
`mondifcor`  
Warning, `jj0cur` is implicitly declared local to procedure  
`mondifcor`  
Warning, `jj1cur` is implicitly declared local to procedure  
`mondifcor`  
Warning, `jj2cur` is implicitly declared local to procedure  
`mondifcor`  
Warning, `jj3cur` is implicitly declared local to procedure  
`mondifcor`

```
> eqren := Array[1..12]:
eqren[1] := reneq(eq5) :
eqren[2] := reneq(eq6) :
eqren[3] := reneq(eq7) :
eqren[4] := reneq(eq8) :
eqren[5] := reneq(eq9) :
eqren[6] := reneq(eq10) :
eqren[7] := reneq(eq11) :
eqren[8] := reneq(eq12) :
eqren[9] := reneq(eq13) :
eqren[10] := reneq(eq14) :
eqren[11] := reneq(eq15) :
eqren[12] := reneq(eq16) :
```

```
> nd2 :=  $\frac{(ktay + 4)!}{4! \cdot (ktay)!}$ ;
```

```
  #number of derivatives with respect to x0,x1,x2,x3 of the total order not greater than ktay
neq := 12;
dreq7 := Array(1..neq, 1..nd2, fill=0) :
numder := 0 :
  for ii0 from 0 to ktay do:
    for ii1 from 0 to ktay do:
      for ii2 from 0 to ktay do:
        for ii3 from 0 to ktay do:
          if ii0 + ii1 + ii2 + ii3 ≤ ktay then numder := numder + 1 :
```



```

        end if:
      end do:
    end do:
  end do:
end do:
number;

```

```

nd2 := 210
neq := 12
210

```

(1.4)

```

> st35 := time( ) :
for ieq from 1 to neq do:#computation of prolongations
  number := 1 :
  for ii0 from 0 to ktay do:
    for ii1 from 0 to ktay do:
      for ii2 from 0 to ktay do:
        for ii3 from 0 to ktay do:
          if ii0 + ii1 + ii2 + ii3 ≤ ktay then dereq7[ieq, number] := add(i38, i38
= map(mondifcor, MonomialList(expand(eqren[ieq])), ii0, ii1, ii2, ii3) ) : number :=
number + 1 :
        end if:
      end do:
    end do:
  end do:
end do:
time( ) - st35;

```

1.641

(1.5)

```

> eqren[1]; eqren[2]; eqren[3]; eqren[4]; eqren[5]; eqren[6]; eqren[7]; eqren[8]; eqren[9];
eqren[10]; eqren[11]; eqren[12];
( psa8, 0, 0, 0, 0 + psa9, 0, 0, 0, 0 ) psa4, 0, 0, 0, 0 + psa11, 0, 0, 0, 0 psa2, 0, 0, 0, 0
+ psa10, 0, 0, 0, 0 psa1, 0, 0, 0, 0 + psa3, 1, 0, 0, 0 - psa1, 0, 1, 0, 0 + psa2, 0, 0, 1, 0 - psa7, 0, 0, 0, 0
- psa3, 0, 0, 0, 1
( psa8, 0, 0, 0, 0 + psa9, 0, 0, 0, 0 ) psa3, 0, 0, 0, 0 + psa11, 0, 0, 0, 0 psa1, 0, 0, 0, 0
- psa10, 0, 0, 0, 0 psa2, 0, 0, 0, 0 + psa1, 0, 0, 1, 0 + psa2, 0, 1, 0, 0 + psa4, 0, 0, 0, 1 - psa4, 1, 0, 0, 0
( psa8, 0, 0, 0, 0 - psa9, 0, 0, 0, 0 ) psa2, 0, 0, 0, 0 + psa11, 0, 0, 0, 0 psa4, 0, 0, 0, 0
- psa10, 0, 0, 0, 0 psa3, 0, 0, 0, 0 - psa4, 0, 0, 1, 0 + psa1, 0, 0, 0, 1 + psa1, 1, 0, 0, 0 - psa6, 0, 0, 0, 0
- psa3, 0, 1, 0, 0
( psa8, 0, 0, 0, 0 - psa9, 0, 0, 0, 0 ) psa1, 0, 0, 0, 0 + psa11, 0, 0, 0, 0 psa3, 0, 0, 0, 0
+ psa10, 0, 0, 0, 0 psa4, 0, 0, 0, 0 + psa4, 0, 1, 0, 0 - psa2, 0, 0, 0, 1 - psa2, 1, 0, 0, 0 - psa5, 0, 0, 0, 0
- psa3, 0, 0, 1, 0
( psa8, 0, 0, 0, 0 - psa9, 0, 0, 0, 0 ) psa7, 0, 0, 0, 0 - psa11, 0, 0, 0, 0 psa6, 0, 0, 0, 0
- psa10, 0, 0, 0, 0 psa5, 0, 0, 0, 0 - psa6, 0, 0, 1, 0 - psa4, 0, 0, 0, 0 + psa5, 0, 1, 0, 0
- psa5, 0, 0, 0, 0 psa11, 0, 0, 0, 0 + psa6, 0, 0, 0, 0 psa10, 0, 0, 0, 0 - psa3, 0, 0, 0, 0 - psa5, 0, 0, 1, 0

```

$$\begin{aligned}
& -psa_{6,0,1,0,0} - psa_{7,0,0,0,1} - psa_{7,1,0,0,0} \\
& (psa_{8,0,0,0,0} + psa_{9,0,0,0,0}) psa_{6,0,0,0,0} - psa_{11,0,0,0,0} psa_{7,0,0,0,0} - psa_{2,0,0,0,0} \\
& + psa_{7,0,0,1,0} - psa_{5,0,0,0,1} + psa_{5,1,0,0,0} \\
& (psa_{8,0,0,0,0} + psa_{9,0,0,0,0}) psa_{5,0,0,0,0} - psa_{10,0,0,0,0} psa_{7,0,0,0,0} - psa_{1,0,0,0,0} \\
& - psa_{7,0,1,0,0} + psa_{6,0,0,0,1} - psa_{6,1,0,0,0} \\
& - psa_{8,0,2,0,0} - psa_{8,0,0,2,0} - psa_{8,0,0,0,2} - psa_{11,1,1,0,0} - psa_{10,1,0,1,0} - psa_{9,1,0,0,1} \\
& - \frac{221}{2410} psa_{7,0,0,0,0}^2 - \frac{221}{2410} psa_{5,0,0,0,0}^2 - \frac{221}{2410} psa_{6,0,0,0,0}^2 - \frac{221}{2410} psa_{3,0,0,0,0}^2 \\
& - \frac{221}{2410} psa_{4,0,0,0,0}^2 - \frac{221}{2410} psa_{1,0,0,0,0}^2 - \frac{221}{2410} psa_{2,0,0,0,0}^2 \\
& - psa_{11,2,0,0,0} + psa_{11,0,0,2,0} + psa_{11,0,0,0,2} - psa_{8,1,1,0,0} - psa_{10,0,1,1,0} - psa_{9,0,1,0,1} \\
& + \frac{221}{1205} psa_{7,0,0,0,0} psa_{6,0,0,0,0} - \frac{221}{1205} psa_{3,0,0,0,0} psa_{1,0,0,0,0} \\
& - \frac{221}{1205} psa_{4,0,0,0,0} psa_{2,0,0,0,0} \\
& - psa_{10,2,0,0,0} + psa_{10,0,2,0,0} + psa_{10,0,0,2,0} - psa_{8,1,0,1,0} - psa_{11,0,1,1,0} - psa_{9,0,0,1,1} \\
& + \frac{221}{1205} psa_{7,0,0,0,0} psa_{5,0,0,0,0} + \frac{221}{1205} psa_{3,0,0,0,0} psa_{2,0,0,0,0} \\
& - \frac{221}{1205} psa_{4,0,0,0,0} psa_{1,0,0,0,0} \\
& - psa_{9,2,0,0,0} + psa_{9,0,2,0,0} + psa_{9,0,0,2,0} - psa_{8,1,0,0,1} - psa_{11,0,1,0,1} - psa_{10,0,0,1,1} \\
& + \frac{221}{2410} psa_{7,0,0,0,0}^2 - \frac{221}{2410} psa_{5,0,0,0,0}^2 - \frac{221}{2410} psa_{6,0,0,0,0}^2 - \frac{221}{2410} psa_{3,0,0,0,0}^2 \\
& - \frac{221}{2410} psa_{4,0,0,0,0}^2 + \frac{221}{2410} psa_{1,0,0,0,0}^2 + \frac{221}{2410} psa_{2,0,0,0,0}^2
\end{aligned} \tag{1.6}$$

ComputeRanking(ivar, dvarnp2, "DegRevLex");

$$\begin{aligned}
& \text{> resnp2} := \text{DifferentialThomasDecomposition}(L1, [e2[0,0,0,0], ps1r[0,0,0,0]]); \\
& \text{resnp2} := [\text{DifferentialSystem}]
\end{aligned} \tag{1.7}$$

> PrintDifferentialSystem(resnp2[1]) :

Equations:

a0:

```

a0[1,0,0,0], [inf,inf,inf,inf], 1, 2*a0[0,0,0,0]*a1[0,0,0,0]*
ps2i[0,0,0,0]-2*a0[0,0,0,0]*a2[0,0,0,0]*ps2r[0,0,0,0]+2*a0[0,
0,0,0]*ps1r[0,0,0,1]+2*a0[0,0,0,0]*ps2i[0,0,1,0]+2*a0[0,0,0,0]
*ps2r[0,1,0,0]+2*a0[0,0,0,0]*ps3i[0,0,0,0]+a0[0,0,0,1]*ps1r[0,
0,0,0]+a0[0,0,1,0]*ps2i[0,0,0,0]+a0[0,1,0,0]*ps2r[0,0,0,0]-a0
[1,0,0,0]*ps1r[0,0,0,0]-2*a1[0,0,0,0]*ps1r[0,1,0,0]-a1[0,0,0,
1]*ps2r[0,0,0,0]-a1[0,1,0,0]*ps1r[0,0,0,0]+a1[1,0,0,0]*ps2r[0,
0,0,0]-2*a2[0,0,0,0]*ps1r[0,0,1,0]-a2[0,0,0,1]*ps2i[0,0,0,0]-
a2[0,0,1,0]*ps1r[0,0,0,0]+a2[1,0,0,0]*ps2i[0,0,0,0]-2*a3[0,0,
0,0]*ps1r[0,0,0,1]-a3[0,0,0,1]*ps1r[0,0,0,0]+a3[0,0,1,0]*ps2i
[0,0,0,0]+a3[0,1,0,0]*ps2r[0,0,0,0]+a3[1,0,0,0]*ps1r[0,0,0,0]

```

a1:

```

a1[2,0,0,0], [inf,inf,inf,inf], 1, 2*a0[0,0,0,0]^2*a1[0,0,0,0]
*ps1r[0,0,0,0]^2-a0[0,0,0,0]*a2[0,0,0,1]*ps1r[0,0,0,0]^2+a0[0,

```

```

0,0,0]*a2[1,0,0,0]*ps1r[0,0,0,0]^2-a0[0,0,1,0]*a3[0,0,0,0]*
ps1r[0,0,0,0]^2+a2[0,0,0,1]*a3[0,0,0,0]*ps1r[0,0,0,0]^2-a2[1,
0,0,0]*a3[0,0,0,0]*ps1r[0,0,0,0]^2-a3[0,0,0,0]*a3[0,0,1,0]*
ps1r[0,0,0,0]^2-a0[0,0,1,0]*ps1r[0,0,0,0]*ps2r[0,0,1,0]-a0[0,
0,1,0]*ps1r[0,0,0,0]*ps3r[0,0,0,0]+a2[0,0,0,1]*ps1r[0,0,0,0]*
ps2r[0,0,1,0]+a2[0,0,0,1]*ps1r[0,0,0,0]*ps3r[0,0,0,0]-a2[1,0,
0,0]*ps1r[0,0,0,0]*ps2r[0,0,1,0]-a2[1,0,0,0]*ps1r[0,0,0,0]
*ps3r[0,0,0,0]-a3[0,0,1,0]*ps1r[0,0,0,0]*ps2r[0,0,1,0]-a3[0,0,
1,0]*ps1r[0,0,0,0]*ps3r[0,0,0,0]-2*ps1r[0,0,0,0]*ps1r[0,0,0,1]
*a0[0,1,0,0]-2*ps1r[0,0,0,0]*ps2i[0,0,1,0]*a0[0,1,0,0]-2*ps1r
[0,0,0,0]*ps2r[0,2,0,0]*a0[0,0,0,0]-3*ps1r[0,0,0,0]*ps2r[0,1,
0,0]*a0[0,1,0,0]-2*ps1r[0,0,0,0]*ps3i[0,1,0,0]*a0[0,0,0,0]-2*
ps1r[0,0,0,0]*ps3i[0,0,0,0]*a0[0,1,0,0]+2*ps1r[0,0,0,0]*a1[0,
1,0,0]*ps1r[0,1,0,0]+2*ps1r[0,0,0,0]*a1[0,0,0,0]*ps1r[0,2,0,0]
+ps1r[0,0,0,0]*a1[0,1,0,1]*ps2r[0,0,0,0]+ps1r[0,0,0,0]*a1[0,0,
0,1]*ps2r[0,1,0,0]+2*ps1r[0,0,0,0]*a2[0,1,0,0]*ps1r[0,0,1,0]
+2*ps1r[0,0,0,0]*a2[0,0,0,0]*ps1r[0,1,1,0]+ps1r[0,0,0,0]*a2[0,
1,0,1]*ps2i[0,0,0,0]+2*ps1r[0,0,0,0]*a0[0,0,0,0]^2*ps1r[0,0,1,
0]-2*ps1r[0,0,0,0]*a0[0,0,0,0]*ps2r[0,0,2,0]-2*ps1r[0,0,0,0]*
a0[0,0,0,0]*ps3r[0,0,1,0]+2*a0[0,0,0,0]*ps1r[0,0,0,1]*ps1r[0,
1,0,0]+2*a0[0,0,0,0]*ps1r[0,1,0,0]*ps2i[0,0,1,0]+2*a0[0,0,0,0]
*ps1r[0,1,0,0]*ps2r[0,1,0,0]+2*a0[0,0,0,0]*ps1r[0,1,0,0]*ps3i
[0,0,0,0]+a0[0,0,1,0]*ps1r[0,1,0,0]*ps2i[0,0,0,0]+a0[0,1,0,0]*
ps1r[0,1,0,0]*ps2r[0,0,0,0]-a1[0,0,0,1]*ps1r[0,1,0,0]*ps2r[0,
0,0,0]+a1[1,0,0,0]*ps1r[0,1,0,0]*ps2r[0,0,0,0]-2*a2[0,0,0,0]*
ps1r[0,0,1,0]*ps1r[0,1,0,0]-a2[0,0,0,1]*ps1r[0,1,0,0]*ps2i[0,
0,0,0]+a2[1,0,0,0]*ps1r[0,1,0,0]*ps2i[0,0,0,0]-2*a3[0,0,0,0]*
ps1r[0,0,0,1]*ps1r[0,1,0,0]+a3[0,0,1,0]*ps1r[0,1,0,0]*ps2i[0,
0,0,0]+a3[0,1,0,0]*ps1r[0,1,0,0]*ps2r[0,0,0,0]+3*a0[0,0,0,0]*
a0[0,0,1,0]*ps1r[0,0,0,0]^2-a0[0,0,0,0]*a3[0,0,1,0]*ps1r[0,0,
0,0]^2-ps1r[0,0,0,0]*ps2i[0,0,0,0]*a0[0,1,1,0]-ps1r[0,0,0,0]*
a1[1,0,0,0]*ps2r[0,1,0,0]-ps1r[0,0,0,0]*a2[1,1,0,0]*ps2i[0,0,
0,0]-ps1r[0,0,0,0]*ps2i[0,0,0,0]*a3[0,1,1,0]-ps1r[0,0,0,0]*
ps2r[0,1,0,0]*a3[0,1,0,0]-ps1r[0,0,0,0]*ps2r[0,0,0,0]*a3[0,2,
0,0]+3*e2[0,0,0,0]*ps1r[0,0,0,0]^3*ps2r[0,0,0,0]+ps1r[0,0,0,0]
*e2[0,0,0,0]*ps2r[0,0,0,0]^3+ps1r[0,0,0,0]*a0[0,0,0,2]*ps2r[0,
0,0,0]+ps1r[0,0,0,0]*a0[0,0,2,0]*ps2r[0,0,0,0]+ps1r[0,0,0,0]*
a2[1,0,1,0]*ps2r[0,0,0,0]+ps1r[0,0,0,0]*a3[1,0,0,1]*ps2r[0,0,
0,0]+2*ps1r[0,0,0,0]*ps1r[0,1,0,1]*a3[0,0,0,0]+2*ps1r[0,0,0,0]
*ps1r[0,0,0,1]*a3[0,1,0,0]-2*ps1r[0,0,0,0]*ps1r[0,1,0,1]*a0[0,
0,0,0]-4*ps1r[0,0,0,0]*a0[0,0,0,0]*a1[0,0,0,0]*ps2r[0,0,1,0]
-2*ps1r[0,0,0,0]*a0[0,0,0,0]*a1[0,0,1,0]*ps2r[0,0,0,0]-2*ps1r
[0,0,0,0]*a0[0,0,0,0]*a2[0,0,0,0]*ps2i[0,0,1,0]-2*ps1r[0,0,0,
0]*a0[0,0,0,0]*a2[0,0,1,0]*ps2i[0,0,0,0]-2*ps1r[0,0,0,0]*a0[0,
0,0,0]*a3[0,0,0,0]*ps1r[0,0,1,0]+ps1r[0,0,0,0]*e2[0,0,0,0]*
ps2i[0,0,0,0]^2*ps2r[0,0,0,0]+ps1r[0,0,0,0]*e2[0,0,0,0]*ps2r
[0,0,0,0]*ps3i[0,0,0,0]^2+ps1r[0,0,0,0]*e2[0,0,0,0]*ps2r[0,0,
0,0]*ps3r[0,0,0,0]^2+ps1r[0,0,0,0]*e2[0,0,0,0]*ps2r[0,0,0,0]*
ps4i[0,0,0,0]^2+ps1r[0,0,0,0]*e2[0,0,0,0]*ps2r[0,0,0,0]*ps4r
[0,0,0,0]^2-2*ps1r[0,0,0,0]*a0[0,1,0,0]*a1[0,0,0,0]*ps2i[0,0,
0,0]-2*ps1r[0,0,0,0]*a0[0,0,0,0]*a1[0,1,0,0]*ps2i[0,0,0,0]+2*
ps1r[0,0,0,0]*a0[0,1,0,0]*a2[0,0,0,0]*ps2r[0,0,0,0]+2*ps1r[0,
0,0,0]*a0[0,0,0,0]*a2[0,1,0,0]*ps2r[0,0,0,0]+2*ps1r[0,0,0,0]*
a0[0,0,0,0]*a2[0,0,0,0]*ps2r[0,1,0,0]-2*e2[0,0,0,0]*ps1r[0,0,
0,0]^2*ps3i[0,0,0,0]*ps4i[0,0,0,0]-2*e2[0,0,0,0]*ps1r[0,0,0,0]
^2*ps3r[0,0,0,0]*ps4r[0,0,0,0]+2*a0[0,0,0,0]*a1[0,0,0,0]*ps1r
[0,1,0,0]*ps2i[0,0,0,0]-2*a0[0,0,0,0]*a2[0,0,0,0]*ps1r[0,1,0,

```

```

0]*ps2r[0,0,0,0]-2*a0[0,0,0,0]*a1[0,0,0,0]^2*ps1r[0,0,0,0]*
ps2r[0,0,0,0]-2*a0[0,0,0,0]*a1[0,0,0,0]*a3[0,0,0,0]*ps1r[0,0,
0,0]^2-2*a0[0,0,0,0]*a1[0,0,0,0]*ps1r[0,0,0,0]*ps3r[0,0,0,0]-
a0[0,0,1,0]*a1[0,0,0,0]*ps1r[0,0,0,0]*ps2r[0,0,0,0]-a0[0,0,1,
0]*a2[0,0,0,0]*ps1r[0,0,0,0]*ps2i[0,0,0,0]+a1[0,0,0,0]*a2[0,0,
0,1]*ps1r[0,0,0,0]*ps2r[0,0,0,0]-a1[0,0,0,0]*a2[1,0,0,0]*ps1r
[0,0,0,0]*ps2r[0,0,0,0]-a1[0,0,0,0]*a3[0,0,1,0]*ps1r[0,0,0,0]*
ps2r[0,0,0,0]+a2[0,0,0,0]*a2[0,0,0,1]*ps1r[0,0,0,0]*ps2i[0,0,
0,0]-a2[0,0,0,0]*a2[1,0,0,0]*ps1r[0,0,0,0]*ps2i[0,0,0,0]-a2[0,
0,0,0]*a3[0,0,1,0]*ps1r[0,0,0,0]*ps2i[0,0,0,0]+a1[0,2,0,0]*
ps1r[0,0,0,0]^2-2*a1[0,0,0,0]*ps1r[0,1,0,0]^2-ps1r[0,0,0,0]^2*
a3[1,1,0,0]-ps1r[0,0,0,0]^2*a0[0,1,0,1]+a1[0,0,0,2]*ps1r[0,0,
0,0]^2+a1[0,0,2,0]*ps1r[0,0,0,0]^2-a1[2,0,0,0]*ps1r[0,0,0,0]^2
-2*a0[0,0,0,0]*a1[0,0,0,0]*a2[0,0,0,0]*ps1r[0,0,0,0]*ps2i[0,0,
0,0]
a1[1,1,0,0], [ 0,inf,inf,inf,], 1, e2[0,0,0,0]*ps1r[0,0,0,0]
^2+e2[0,0,0,0]*ps2i[0,0,0,0]^2+e2[0,0,0,0]*ps2r[0,0,0,0]^2+e2
[0,0,0,0]*ps3i[0,0,0,0]^2+e2[0,0,0,0]*ps3r[0,0,0,0]^2+e2[0,0,
0,0]*ps4i[0,0,0,0]^2+e2[0,0,0,0]*ps4r[0,0,0,0]^2+a0[0,0,0,2]+
a0[0,0,2,0]+a0[0,2,0,0]+a1[1,1,0,0]+a2[1,0,1,0]+a3[1,0,0,1]
ps4i:
ps4i[1,0,0,0], [inf,inf,inf,inf,], 1, a0[0,0,0,0]*ps4r[0,0,0,0]
+a1[0,0,0,0]*ps3r[0,0,0,0]-a2[0,0,0,0]*ps3i[0,0,0,0]-a3[0,0,0,
0]*ps4r[0,0,0,0]-ps2r[0,0,0,0]-ps3i[0,1,0,0]-ps3r[0,0,1,0]+
ps4i[0,0,0,1]+ps4i[1,0,0,0]
ps4r:
ps4r[1,0,0,0], [inf,inf,inf,inf,], 1, a0[0,0,0,0]*ps4i[0,0,0,0]
+a1[0,0,0,0]*ps3i[0,0,0,0]+a2[0,0,0,0]*ps3r[0,0,0,0]-a3[0,0,0,
0]*ps4i[0,0,0,0]-ps2i[0,0,0,0]-ps3i[0,0,1,0]+ps3r[0,1,0,0]-
ps4r[0,0,0,1]-ps4r[1,0,0,0]
ps3i:
ps3i[1,0,0,0], [inf,inf,inf,inf,], 1, a0[0,0,0,0]*ps3r[0,0,0,0]
+a1[0,0,0,0]*ps4r[0,0,0,0]+a2[0,0,0,0]*ps4i[0,0,0,0]+a3[0,0,0,
0]*ps3r[0,0,0,0]-ps1r[0,0,0,0]-ps3i[0,0,0,1]+ps3i[1,0,0,0]-
ps4i[0,1,0,0]+ps4r[0,0,1,0]
ps3r:
ps3r[1,0,0,0], [inf,inf,inf,inf,], 1, a0[0,0,0,0]*ps3i[0,0,0,0]
+a1[0,0,0,0]*ps4i[0,0,0,0]-a2[0,0,0,0]*ps4r[0,0,0,0]+a3[0,0,0,
0]*ps3i[0,0,0,0]+ps3r[0,0,0,1]-ps3r[1,0,0,0]+ps4i[0,0,1,0]+
ps4r[0,1,0,0]
ps2i:
ps2i[1,0,0,0], [inf,inf,inf,inf,], 1, a0[0,0,0,0]*ps2r[0,0,0,0]
-a1[0,0,0,0]*ps1r[0,0,0,0]+a3[0,0,0,0]*ps2r[0,0,0,0]+ps1r[0,0,
1,0]-ps2i[0,0,0,1]+ps2i[1,0,0,0]-ps4r[0,0,0,0]
ps2i[0,1,0,0], [ 0,inf,inf,inf,], 1, a0[0,0,0,0]*ps1r[0,0,0,0]
-a1[0,0,0,0]*ps2r[0,0,0,0]-a2[0,0,0,0]*ps2i[0,0,0,0]-a3[0,0,0,
0]*ps1r[0,0,0,0]+ps2i[0,1,0,0]-ps2r[0,0,1,0]-ps3r[0,0,0,0]
ps2r:
ps2r[1,0,0,0], [inf,inf,inf,inf,], 1, a0[0,0,0,0]*ps2i[0,0,0,0]
-a2[0,0,0,0]*ps1r[0,0,0,0]+a3[0,0,0,0]*ps2i[0,0,0,0]-ps1r[0,1,
0,0]+ps2r[0,0,0,1]-ps2r[1,0,0,0]-ps4i[0,0,0,0]
ps1r:
ps1r[1,0,0,0], [inf,inf,inf,inf,], 1, a1[0,0,0,0]*ps2i[0,0,0,0]
-a2[0,0,0,0]*ps2r[0,0,0,0]+ps1r[0,0,0,1]+ps1r[1,0,0,0]+ps2i[0,
0,1,0]+ps2r[0,1,0,0]+ps3i[0,0,0,0]
a3:
a3[2,0,0,0], [inf,inf,inf,inf,], 1, -ps1r[0,0,0,0]^2*a3[0,0,0,

```

```

2]-e2[0,0,0,0]*ps1r[0,0,0,0]^4-a3[0,0,2,0]*ps1r[0,0,0,0]^2-a3
[0,2,0,0]*ps1r[0,0,0,0]^2+a3[2,0,0,0]*ps1r[0,0,0,0]^2+ps1r[0,
0,0,0]^2*a3[1,0,0,1]+ps1r[0,0,0,0]^2*a0[0,0,0,2]-2*a0[0,0,0,0]
*ps1r[0,0,0,1]^2+2*a3[0,0,0,0]*ps1r[0,0,0,1]^2+2*ps1r[0,0,0,0]
*a0[0,0,0,1]*a1[0,0,0,0]*ps2i[0,0,0,0]+2*ps1r[0,0,0,0]*a0[0,0,
0,0]*a1[0,0,0,1]*ps2i[0,0,0,0]+2*ps1r[0,0,0,0]*a0[0,0,0,0]*a1
[0,0,0,0]*ps2i[0,0,0,1]-2*ps1r[0,0,0,0]*a0[0,0,0,1]*a2[0,0,0,
0]*ps2r[0,0,0,0]-2*ps1r[0,0,0,0]*a0[0,0,0,0]*a2[0,0,0,0]*ps2r[0,0,0,
1]-2*a0[0,0,0,0]*a1[0,0,0,0]*ps1r[0,0,0,1]*ps2i[0,0,0,0]+2*a0
[0,0,0,0]*a2[0,0,0,0]*ps1r[0,0,0,1]*ps2r[0,0,0,0]+2*a2[0,0,0,
0]*ps1r[0,0,0,1]*ps1r[0,0,1,0]+a2[0,0,0,1]*ps1r[0,0,0,1]*ps2i
[0,0,0,0]-a2[1,0,0,0]*ps1r[0,0,0,1]*ps2i[0,0,0,0]-a3[0,0,1,0]*
ps1r[0,0,0,1]*ps2i[0,0,0,0]-a3[0,1,0,0]*ps1r[0,0,0,1]*ps2r[0,
0,0,0]+2*ps1r[0,0,0,0]*ps1r[0,0,0,2]*a0[0,0,0,0]+2*ps1r[0,0,0,
0]*ps1r[0,0,0,1]*a0[0,0,0,1]+2*ps1r[0,0,0,0]*ps2i[0,0,1,1]*a0
[0,0,0,0]+2*ps1r[0,0,0,0]*ps2i[0,0,1,0]*a0[0,0,0,1]+2*ps1r[0,
0,0,0]*ps2r[0,1,0,1]*a0[0,0,0,0]+2*ps1r[0,0,0,0]*ps2r[0,1,0,0]
*a0[0,0,0,1]+2*ps1r[0,0,0,0]*ps3i[0,0,0,1]*a0[0,0,0,0]+2*ps1r
[0,0,0,0]*ps3i[0,0,0,0]*a0[0,0,0,1]-2*ps1r[0,0,0,0]*a1[0,0,0,
1]*ps1r[0,1,0,0]-2*ps1r[0,0,0,0]*a1[0,0,0,0]*ps1r[0,1,0,1]-
ps1r[0,0,0,0]*a1[0,0,0,2]*ps2r[0,0,0,0]-ps1r[0,0,0,0]*a1[0,0,
0,1]*ps2r[0,0,0,1]-2*ps1r[0,0,0,0]*a2[0,0,0,1]*ps1r[0,0,1,0]
-2*ps1r[0,0,0,0]*a2[0,0,0,0]*ps1r[0,0,1,1]-ps1r[0,0,0,0]*a2[0,
0,0,2]*ps2i[0,0,0,0]-ps1r[0,0,0,0]*a2[0,0,0,1]*ps2i[0,0,0,1]
-2*ps1r[0,0,0,0]*ps1r[0,0,0,2]*a3[0,0,0,0]-2*ps1r[0,0,0,0]*
ps1r[0,0,0,1]*a3[0,0,0,1]+ps1r[0,0,0,0]*a2[1,0,0,1]*ps2i[0,0,
0,0]+ps1r[0,0,0,0]*a2[1,0,0,0]*ps2i[0,0,0,1]+ps1r[0,0,0,0]*
ps2i[0,0,0,1]*a3[0,0,1,0]+ps1r[0,0,0,0]*ps2i[0,0,0,0]*a3[0,0,
1,1]+ps1r[0,0,0,0]*ps2r[0,0,0,1]*a3[0,1,0,0]+ps1r[0,0,0,0]*
ps2r[0,0,0,0]*a3[0,1,0,1]+e2[0,0,0,0]*ps1r[0,0,0,0]^2*ps2i[0,
0,0,0]^2+e2[0,0,0,0]*ps1r[0,0,0,0]^2*ps2r[0,0,0,0]^2+e2[0,0,0,
0]*ps1r[0,0,0,0]^2*ps3i[0,0,0,0]^2+e2[0,0,0,0]*ps1r[0,0,0,0]
^2*ps3r[0,0,0,0]^2-e2[0,0,0,0]*ps1r[0,0,0,0]^2*ps4i[0,0,0,0]^2
-e2[0,0,0,0]*ps1r[0,0,0,0]^2*ps4r[0,0,0,0]^2+ps1r[0,0,0,0]*
ps2i[0,0,0,1]*a0[0,0,1,0]+ps1r[0,0,0,0]*ps2i[0,0,0,0]*a0[0,0,
1,1]+ps1r[0,0,0,0]*ps2r[0,0,0,1]*a0[0,1,0,0]+ps1r[0,0,0,0]*
ps2r[0,0,0,0]*a0[0,1,0,1]+ps1r[0,0,0,0]*a1[1,0,0,1]*ps2r[0,0,
0,0]+ps1r[0,0,0,0]*a1[1,0,0,0]*ps2r[0,0,0,1]-2*a0[0,0,0,0]*
ps1r[0,0,0,1]*ps2i[0,0,1,0]-2*a0[0,0,0,0]*ps1r[0,0,0,1]*ps2r
[0,1,0,0]-2*a0[0,0,0,0]*ps1r[0,0,0,1]*ps3i[0,0,0,0]-a0[0,0,1,
0]*ps1r[0,0,0,1]*ps2i[0,0,0,0]-a0[0,1,0,0]*ps1r[0,0,0,1]*ps2r
[0,0,0,0]+2*a1[0,0,0,0]*ps1r[0,0,0,1]*ps1r[0,1,0,0]+a1[0,0,0,
1]*ps1r[0,0,0,1]*ps2r[0,0,0,0]-a1[1,0,0,0]*ps1r[0,0,0,1]*ps2r
[0,0,0,0]

```

a2:

```

a2[2,0,0,0], [inf,inf,inf,inf,], 1, -2*e2[0,0,0,0]*ps1r[0,0,0,
0]^3*ps2i[0,0,0,0]+ps1r[0,0,0,0]*ps2i[0,0,0,0]*a0[0,0,2,0]+
ps1r[0,0,0,0]*ps2r[0,0,1,0]*a0[0,1,0,0]+ps1r[0,0,0,0]*ps2r[0,
0,0,0]*a0[0,1,1,0]+ps1r[0,0,0,0]*a1[1,0,1,0]*ps2r[0,0,0,0]+
ps1r[0,0,0,0]*a1[1,0,0,0]*ps2r[0,0,1,0]+ps1r[0,0,0,0]*a2[1,0,
1,0]*ps2i[0,0,0,0]+ps1r[0,0,0,0]*a2[1,0,0,0]*ps2i[0,0,1,0]+
ps1r[0,0,0,0]*ps2i[0,0,1,0]*a3[0,0,1,0]+ps1r[0,0,0,0]*ps2i[0,
0,0,0]*a3[0,0,2,0]+ps1r[0,0,0,0]*ps2r[0,0,1,0]*a3[0,1,0,0]+
ps1r[0,0,0,0]*ps2r[0,0,0,0]*a3[0,1,1,0]-2*ps1r[0,0,0,0]*a1[0,
0,1,0]*ps1r[0,1,0,0]-2*ps1r[0,0,0,0]*a1[0,0,0,0]*ps1r[0,1,1,0]
-ps1r[0,0,0,0]*a1[0,0,1,1]*ps2r[0,0,0,0]-ps1r[0,0,0,0]*a1[0,0,

```

```

0,1]*ps2r[0,0,1,0]-2*ps1r[0,0,0,0]*a2[0,0,1,0]*ps1r[0,0,1,0]
-2*ps1r[0,0,0,0]*a2[0,0,0,0]*ps1r[0,0,2,0]-ps1r[0,0,0,0]*a2[0,
0,1,1]*ps2i[0,0,0,0]-ps1r[0,0,0,0]*a2[0,0,0,1]*ps2i[0,0,1,0]
-2*ps1r[0,0,0,0]*ps1r[0,0,1,1]*a3[0,0,0,0]-2*ps1r[0,0,0,0]*
ps1r[0,0,0,1]*a3[0,0,1,0]+2*ps1r[0,0,0,0]*ps1r[0,0,1,1]*a0[0,
0,0,0]+2*ps1r[0,0,0,0]*ps1r[0,0,0,1]*a0[0,0,1,0]+2*ps1r[0,0,0,
0]*ps2i[0,0,2,0]*a0[0,0,0,0]+3*ps1r[0,0,0,0]*ps2i[0,0,1,0]*a0
[0,0,1,0]+2*ps1r[0,0,0,0]*ps2r[0,1,1,0]*a0[0,0,0,0]+2*ps1r[0,
0,0,0]*ps2r[0,1,0,0]*a0[0,0,1,0]+2*ps1r[0,0,0,0]*ps3i[0,0,1,0]
*a0[0,0,0,0]+2*ps1r[0,0,0,0]*ps3i[0,0,0,0]*a0[0,0,1,0]-2*a0[0,
0,0,0]*ps1r[0,0,0,1]*ps1r[0,0,1,0]-2*a0[0,0,0,0]*ps1r[0,0,1,0]
*ps2i[0,0,1,0]-2*a0[0,0,0,0]*ps1r[0,0,1,0]*ps2r[0,1,0,0]-2*a0
[0,0,0,0]*ps1r[0,0,1,0]*ps3i[0,0,0,0]-a0[0,0,1,0]*ps1r[0,0,1,
0]*ps2i[0,0,0,0]-a0[0,1,0,0]*ps1r[0,0,1,0]*ps2r[0,0,0,0]+2*a1
[0,0,0,0]*ps1r[0,0,1,0]*ps1r[0,1,0,0]+a1[0,0,0,1]*ps1r[0,0,1,
0]*ps2r[0,0,0,0]-a1[1,0,0,0]*ps1r[0,0,1,0]*ps2r[0,0,0,0]+a2[0,
0,0,1]*ps1r[0,0,1,0]*ps2i[0,0,0,0]-a2[1,0,0,0]*ps1r[0,0,1,0]*
ps2i[0,0,0,0]+2*a3[0,0,0,0]*ps1r[0,0,0,1]*ps1r[0,0,1,0]-a3[0,
0,1,0]*ps1r[0,0,1,0]*ps2i[0,0,0,0]-a3[0,1,0,0]*ps1r[0,0,1,0]*
ps2r[0,0,0,0]+ps1r[0,0,0,0]^2*a0[0,0,1,1]+ps1r[0,0,0,0]^2*a3
[1,0,1,0]-a2[0,0,0,2]*ps1r[0,0,0,0]^2-a2[0,2,0,0]*ps1r[0,0,0,
0]^2+a2[2,0,0,0]*ps1r[0,0,0,0]^2-a2[0,0,2,0]*ps1r[0,0,0,0]
^2+2*a2[0,0,0,0]*ps1r[0,0,1,0]^2-2*ps1r[0,0,0,0]*a0[0,0,0,0]*
a2[0,0,1,0]*ps2r[0,0,0,0]-2*ps1r[0,0,0,0]*a0[0,0,0,0]*a2[0,0,
0,0]*ps2r[0,0,1,0]+2*ps1r[0,0,0,0]*a0[0,0,1,0]*a1[0,0,0,0]*
ps2i[0,0,0,0]+2*ps1r[0,0,0,0]*a0[0,0,0,0]*a1[0,0,1,0]*ps2i[0,
0,0,0]+2*ps1r[0,0,0,0]*a0[0,0,0,0]*a1[0,0,0,0]*ps2i[0,0,1,0]
-2*ps1r[0,0,0,0]*a0[0,0,1,0]*a2[0,0,0,0]*ps2r[0,0,0,0]-2*e2[0,
0,0,0]*ps1r[0,0,0,0]^2*ps3i[0,0,0,0]*ps4r[0,0,0,0]+2*e2[0,0,0,
0]*ps1r[0,0,0,0]^2*ps3r[0,0,0,0]*ps4i[0,0,0,0]-2*a0[0,0,0,0]*
a1[0,0,0,0]*ps1r[0,0,1,0]*ps2i[0,0,0,0]+2*a0[0,0,0,0]*a2[0,0,
0,0]*ps1r[0,0,1,0]*ps2r[0,0,0,0]
e2:
e2[1,0,0,0], [inf,inf,inf,inf], 1, e2[1,0,0,0]
e2[0,1,0,0], [ 0,inf,inf,inf], 1, e2[0,1,0,0]
e2[0,0,1,0], [ 0, 0,inf,inf], 1, e2[0,0,1,0]
e2[0,0,0,1], [ 0, 0, 0,inf], 1, e2[0,0,0,1]
Inequations:
e2[0,0,0,0], 1: e2[0,0,0,0]
ps1r[0,0,0,0], 1: ps1r[0,0,0,0]

```

```
nine := rand(1..9) : one := rand(0..1) :
```

```
nine2( ) :=  $\frac{\text{nine}( ) \cdot (2 \cdot \text{one}( ) - 1)}{\text{nine}( )}$  :
```

```
nine2( )
```

*#function nine2: nominator and denominator are random integer numbers from 1 to 9, the sign is also random*

*#this function is used to assign values to derivatives of a particular solution*

$$-\frac{1}{4}$$

(45)

```

> ndp2 :=  $\frac{(ktay + 2 + 4)!}{(ktay + 2)! \cdot 4!}$ ;
nun := 11;

```

#number of derivatives of orders from 0 to ktay+2 of a function depending on 4 independent variables

*ndp2 := 495*

*nun := 11*

(46)

> derivrat := Array(1..ndp2, 1..nun, fill=0);

*derivrat :=*  $\left[ \begin{array}{l} 1..495 \times 1..11 \text{ Array} \\ \text{Data Type: anything} \\ \text{Storage: rectangular} \\ \text{Order: Fortran\_order} \end{array} \right]$

(47)

*der := Array(0..3, 1..ndp2, fill=0) : count1 := 1 : ii := Array(0..ktay+2, 0..ktay+2, 0..ktay+2, 0..ktay+2, fill=0) :*

> *nun := 11 : iip2 := Array(1..ndp2, 1..nun, fill=0) :*

**for ii0 from 0 to ktay+2 do**

**for ii1 from 0 to ktay+2 do for ii2 from 0 to ktay+2 do for ii3 from 0 to ktay+2 do if ii0 + ii1 + ii2 + ii3 ≤ ktay+2 then ii[ii0, ii1, ii2, ii3] := count1 : der[0, count1] := ii0 : der[1, count1] := ii1 : der[2, count1] := ii2 : der[3, count1] := ii3 : count1 := count1 + 1 : end if : end do: end do: end do: end do:**

#derivative of orders ii0,ii1,ii2,ii3 with respect to x0,x1,x2,x3 has number ii[ii0, ii1, ii2, ii3]

> *stt1 := time( ) :*

*count2 := 0 :*

**for ii1 from 0 to ktay+2 do for ii2 from 0 to ktay+2 do for ii3 from 0 to ktay+2 do if ii1 + ii2 + ii3 ≤ ktay+2 then #print(ii0, ii1, ii2, ii3);**

*count2 := count2 + 1 : end if : end do: end do: end do: count2;*

*#ArrayDims(derivrat);*

*#ArrayDims(ii); ArrayDims(iip2); ktay, nd; nun;*

*#max(ii); min(ii);*

*#count2 - number of derivatives with ii0=0*

**while count2 > 0**

**do for ii1 from 0 to ktay+2**

**do for ii2 from 0 to ktay+2**

**do for ii3 from 0 to ktay+2**

**do if ii1 + ii2 + ii3 ≤ ktay+2 then**

*#print(count2, ii0, ii1, ii2, ii3, ii[0, ii1, ii2, ii3]);*

*derivrat[ii[0, ii1, ii2, ii3], 8] := nine2( ) :*

*iip2[ii[0, ii1, ii2, ii3], 8] := 1 :*

*derivrat[ii[0, ii1, ii2, ii3], 11] := nine2( ) :*

*iip2[ii[0, ii1, ii2, ii3], 11] := 1 :*

*derivrat[ii[0, ii1, ii2, ii3], 1] := nine2( ) :*

*iip2[ii[0, ii1, ii2, ii3], 1] := 1 :*

*derivrat[ii[0, ii1, ii2, ii3], 2] := nine2( ) :*

*iip2[ii[0, ii1, ii2, ii3], 2] := 1 :*

*derivrat[ii[0, ii1, ii2, ii3], 3] := nine2( ) :*

*iip2[ii[0, ii1, ii2, ii3], 3] := 1 :*

*derivrat[ii[0, ii1, ii2, ii3], 4] := nine2( ) :*

*iip2[ii[0, ii1, ii2, ii3], 4] := 1 :*

*derivrat[ii[0, ii1, ii2, ii3], 6] := nine2( ) :*

*iip2[ii[0, ii1, ii2, ii3], 6] := 1 :*

*derivrat[ii[0, ii1, ii2, ii3], 7] := nine2( ) :*

```

iip2[ii[0, ii1, ii2, ii3], 7] := 1 :
derivrat[ii[0, ii1, ii2, ii3], 9] := nine2( ) :
iip2[ii[0, ii1, ii2, ii3], 9] := 1 :
derivrat[ii[0, ii1, ii2, ii3], 10] := nine2( ) :
iip2[ii[0, ii1, ii2, ii3], 10] := 1 :
count2 := count2 - 1 :
end if :
end do:
end do:
end do:
end do:
#derivatives with ii0=0 are assigned random rational values for a particular solution
delttt1 := time( ) - stt1;

```

$$\frac{165}{delttt1} := 0.031 \quad (48)$$

```
> derivrat[1, 1];
```

$$-\frac{7}{3} \quad (49)$$

```

> stt2 := time( ) :
count2 := 0 :
for ii1 from 0 to ktay + 2 do for ii2 from 0 to ktay + 2 do for ii3 from 0 to ktay + 2 do if 1 + ii1
+ ii2 + ii3 ≤ ktay + 2 then #print(ii0, ii1, ii2, ii3);
count2 := count2 + 1 : end if : end do: end do: end do: count2;
while count2 > 0
do for ii1 from 0 to ktay + 2
do for ii2 from 0 to ktay + 2
do for ii3 from 0 to ktay + 2
do if 1 + ii1 + ii2 + ii3 ≤ ktay + 2 then
derivrat[ii[1, ii1, ii2, ii3], 9] := nine2( ) :
iip2[ii[1, ii1, ii2, ii3], 9] := 1 :
derivrat[ii[1, ii1, ii2, ii3], 10] := nine2( ) :
iip2[ii[1, ii1, ii2, ii3], 10] := 1 :
count2 := count2 - 1 :
end if :
end do:
end do:
end do:
end do:
#derivatives with ii0=1 are assigned random rational values for a particular solution
delttt2 := time( ) - stt2;

```

$$\frac{120}{delttt2} := 0.016 \quad (50)$$

```

> stt3 := time( ) :
count2 := 0 :
for ii2 from 0 to ktay + 2 do for ii3 from 0 to ktay + 2 do if ii2 + ii3 ≤ ktay + 2 then
#print(ii0, ii1, ii2, ii3);
count2 := count2 + 1 : end if : end do: end do: count2;
while count2 > 0
do for ii2 from 0 to ktay + 2
do for ii3 from 0 to ktay + 2

```



```

        do if  $ii2 + ii3 \leq ktay + 2$  then
            derivrat[ii[0, 0, ii2, ii3], 5] := nine2( ) :
            iip2[ii[0, 0, ii2, ii3], 5] := 1 :
            count2 := count2 - 1 :
        end if :
    end do:
end do:
end do:
end do:
#some derivatives with  $ii0=1$  are assigned random rational values for a particular solution
delttt3 := time( ) - stt3;

```

45

delttt3 := 0.

(51)

```

> stt3a := time( ) :
count2 := 0 :
for ii2 from 0 to ktay + 2 do for ii3 from 0 to ktay + 2 do if  $1 + ii2 + ii3 \leq ktay + 2$  then
    #print(ii0, ii1, ii2, ii3);
count2 := count2 + 1 : end if : end do: end do: count2;
while count2 > 0
    do for ii2 from 0 to ktay + 2
        do for ii3 from 0 to ktay + 2
            do if  $1 + ii2 + ii3 \leq ktay + 2$  then
                derivrat[ii[1, 0, ii2, ii3], 11] := nine2( ) :
                iip2[ii[1, 0, ii2, ii3], 11] := 1 :
                count2 := count2 - 1 :
            end if :
        end do:
    end do:
end do:
#some derivatives with  $ii0=1$  are assigned random rational values for a particular solution
delttt3a := time( ) - stt3a;

```

36

delttt3a := 0.

(52)

```

> iinext := Array(0..ktay, 0..ktay, 0..ktay, 0..ktay, fill = 0) :
countnext := 1 :
for ii0 from 0 to ktay do
    for ii1 from 0 to ktay do
        for ii2 from 0 to ktay do
            for ii3 from 0 to ktay do
                if  $ii0 + ii1 + ii2 + ii3 \leq ktay$  then
                    iinext[ii0, ii1, ii2, ii3] := countnext :
                    countnext := countnext + 1 :
                end if:
            end do:
        end do:
    end do:
end do:
countnext;

```

211

(53)

```

> dereqint := Array(1..neq, 1..nd2, fill = 0) :
for ineq from 1 to neq do:

```

```
    for ind2 from 1 to nd2 do:  
        dereqint[ineq, ind2] := dereq7[ineq, ind2]:  
    end do:  
end do:  
ArrayDims(dereqint);
```

```

> ArrayDims(iip2);
countiip21 := 0 :
for inun from 1 to nun do:
  for ii0 from 0 to ktay + 2 do:
    for ii1 from 0 to ktay + 2 do:
      for ii2 from 0 to ktay + 2 do:
        for ii3 from 0 to ktay + 2 do:
          if ii0 + ii1 + ii2 + ii3 ≤ ktay + 2 and iip2[ii[ii0, ii1, ii2, ii3], inun] = 1
        then
          countiip21 := countiip21 + 1 :
        end if:
      end do:
    end do:
  end do:
end do:
countiip21;
arii1 := Array[1..countiip21] : brii1 := Array[1..countiip21] :
countiip21 := 1 :
for inun from 1 to nun do:
  for ii0 from 0 to ktay + 2 do:
    for ii1 from 0 to ktay + 2 do:
      for ii2 from 0 to ktay + 2 do:
        for ii3 from 0 to ktay + 2 do:
          if ii0 + ii1 + ii2 + ii3 ≤ ktay + 2 and iip2[ii[ii0, ii1, ii2, ii3], inun] = 1
        then
          arii1[countiip21] := psa[inun, ii0, ii1, ii2, ii3] :
          brii1[countiip21] := derivrat[ii[ii0, ii1, ii2, ii3], inun] :
          countiip21 := countiip21 + 1 :
        end if:
      end do:
    end do:
  end do:
end do:
end do:

```

```

> eqns := {seq(arii1[vvv] = brii1[vvv], vvv = 1..countiip21)} :
#equations to build the particular solution
> for ineq from 1 to neq do:
  numder := 1 :
  for ii0 from 0 to ktay do:
    for ii1 from 0 to ktay do:
      for ii2 from 0 to ktay do:
        for ii3 from 0 to ktay do:
          if ii0 + ii1 + ii2 + ii3 ≤ ktay then
            dereqint[ineq, numder] := eval(dereqint[ineq, numder], eqns);
          numder := numder + 1 :
        end if:
      end do:
    end do:
  end do:
end do:

```

```

        end do:
      end do:
    end do:
  end do:
> ifinish := 0;#building the particular solution
  countloop := 1 :
  while ifinish = 0 do:
    countloop := countloop + 1 :
    for inun from 1 to nun do:
      for ii0 from 0 to ktay do:
        for ii1 from 0 to ktay do:
          for ii2 from 0 to ktay do:
            for ii3 from 0 to ktay do:
              if ii0 + ii1 + ii2 + ii3 ≤ ktay then
                if iip2[ii[ii0, ii1, ii2, ii3], inun] = 0 then
                  if inun = 1 then dereqint[3, iinext[ii0 - 1, ii1, ii2, ii3]] :=
eval(dereqint[3, iinext[ii0 - 1, ii1, ii2, ii3]], eqns) : eqcur := dereqint[3, iinext[ii0 - 1, ii1,
ii2, ii3]] :
                  elif inun = 2 then dereqint[4, iinext[ii0 - 1, ii1, ii2, ii3]] :=
eval(dereqint[4, iinext[ii0 - 1, ii1, ii2, ii3]], eqns) : eqcur := dereqint[4, iinext[ii0 - 1, ii1,
ii2, ii3]] :
                  elif inun = 3 then dereqint[1, iinext[ii0 - 1, ii1, ii2, ii3]] :=
eval(dereqint[1, iinext[ii0 - 1, ii1, ii2, ii3]], eqns) : eqcur := dereqint[1, iinext[ii0 - 1, ii1,
ii2, ii3]] :
                  elif inun = 4 then dereqint[2, iinext[ii0 - 1, ii1, ii2, ii3]] :=
eval(dereqint[2, iinext[ii0 - 1, ii1, ii2, ii3]], eqns) : eqcur := dereqint[2, iinext[ii0 - 1, ii1,
ii2, ii3]] :
                  elif inun = 6 then dereqint[8, iinext[ii0 - 1, ii1, ii2, ii3]] :=
eval(dereqint[8, iinext[ii0 - 1, ii1, ii2, ii3]], eqns) : eqcur := dereqint[8, iinext[ii0 - 1, ii1,
ii2, ii3]] :
                  elif inun = 7 then dereqint[6, iinext[ii0 - 1, ii1, ii2, ii3]] :=
eval(dereqint[6, iinext[ii0 - 1, ii1, ii2, ii3]], eqns) : eqcur := dereqint[6, iinext[ii0 - 1, ii1,
ii2, ii3]] :
                  elif inun = 9 then dereqint[12, iinext[ii0 - 2, ii1, ii2, ii3]] :=
eval(dereqint[12, iinext[ii0 - 2, ii1, ii2, ii3]], eqns) : eqcur := dereqint[12, iinext[ii0 - 2,
ii1, ii2, ii3]] :
                  #if ii0=1 and ii1=1 and ii2=0 and ii3=0 then
                    #print(countloop, eqcur) :
                  #end if:
                  elif inun = 10 then dereqint[11, iinext[ii0 - 2, ii1, ii2, ii3]] :=
eval(dereqint[11, iinext[ii0 - 2, ii1, ii2, ii3]], eqns) : eqcur := dereqint[11, iinext[ii0 - 2,
ii1, ii2, ii3]] :
                  elif inun = 8 then dereqint[5, iinext[ii0, ii1, ii2, ii3]] :=
eval(dereqint[5, iinext[ii0, ii1, ii2, ii3]], eqns) : eqcur := dereqint[5, iinext[ii0, ii1, ii2, ii3]] :
                  elif inun = 11 and ii0 = 1 then dereqint[9, iinext[ii0 - 1, ii1 - 1, ii2,
ii3]] := eval(dereqint[9, iinext[ii0 - 1, ii1 - 1, ii2, ii3]], eqns) : eqcur := dereqint[9,
iinext[ii0 - 1, ii1 - 1, ii2, ii3]] :
                  elif inun = 11 and ii0 > 1 then dereqint[10, iinext[ii0 - 2, ii1, ii2,
ii3]] := eval(dereqint[10, iinext[ii0 - 2, ii1, ii2, ii3]], eqns) : eqcur := dereqint[10,
iinext[ii0 - 2, ii1, ii2, ii3]] :

```



> ktay;  
6 (57)

> ok := 0  
ok := 0 (58)

> ok := 0;#checking that prolongation equations are satisfied for the particular solution  
for ineq from 1 to neq do:  
  for ii0 from 0 to ktay do:  
    for ii1 from 0 to ktay do:  
      for ii2 from 0 to ktay do:  
        for ii3 from 0 to ktay do:  
          if ii0 + ii1 + ii2 + ii3 < ktay - 2 or (ii0 + ii1 + ii2 + ii3 = ktay - 1  
and ineq ≤ 8) then  
          if eval(dereq7[ineq, iinext[ii0, ii1, ii2, ii3]], eqns) ≠ 0 then  
            ok := 1 : print(ineq, ii0, ii1, ii2, ii3) :  
          end if:  
          end if:  
        end do:  
      end do:  
    end do:  
  end do:  
end do:  
ok;

ok := 0  
1, 5, 0, 0, 0  
2, 5, 0, 0, 0  
3, 5, 0, 0, 0  
4, 5, 0, 0, 0  
7, 5, 0, 0, 0  
8, 5, 0, 0, 0  
1 (59)

> #Only equations with derivatives of greater order than 5 are not satisfied

> ok;  
1 (60)

> time( );  
4987.453 (61)

> nm1 :=  $\frac{(ktay - 1 + 4)!}{(ktay - 1)!4!}$ ;  
iim1 := Array(0..ktay - 1, 0..ktay - 1, 0..ktay - 1, 0..ktay - 1, fill = 0) :  
countm1 := 1;  
  for ii0 from 0 to ktay - 1 do:  
    for ii1 from 0 to ktay - 1 do:  
      for ii2 from 0 to ktay - 1 do:  
        for ii3 from 0 to ktay - 1 do:  
          if ii0 + ii1 + ii2 + ii3 ≤ ktay - 1 then  
            iim1[ii0, ii1, ii2, ii3] := countm1 : countm1 := countm1 + 1 :  
          end if:  
        end do:  
      end do:  
    end do:  
  end do:

```

    end do:
  end do:
  print("loop") :
  nunps := 7 :
  divlin9 := array(1..nm1, 1..nunps) :
  linrat2 := proc(a82)
    #procedure for linearization: A - from the particular solution, psi from the particular solution
    plus variation
    global delt:
    indn := op(1, a82) :
    ind0 := op(2, a82) :
    ind1 := op(3, a82) :
    ind2 := op(4, a82) :
    ind3 := op(5, a82) :
    if indn ≤ 7 then
      derivrat[ii[ind0, ind1, ind2, ind3], indn] + delt·divlin9[iim1[ind0, ind1, ind2, ind3],
      indn] :
    else derivrat[ii[ind0, ind1, ind2, ind3], indn] :
    end if:
  end proc:

```

nm1 := 126

countm1 := 1

"loop"

Warning, `indn` is implicitly declared local to procedure  
`linrat2`  
Warning, `ind0` is implicitly declared local to procedure  
`linrat2`  
Warning, `ind1` is implicitly declared local to procedure  
`linrat2`  
Warning, `ind2` is implicitly declared local to procedure  
`linrat2`  
Warning, `ind3` is implicitly declared local to procedure  
`linrat2`

```

> countm12 := 0 :
  for ineq from 1 to neq do:
    if ineq ≤ 8 then
      ktaycur := ktay - 2 :
    else ktaycur := ktay - 3 :
    end if:
    for ii0 from 0 to ktaycur do:
      for ii1 from 0 to ktaycur do:
        for ii2 from 0 to ktaycur do:
          for ii3 from 0 to ktaycur do:
            if ii0 + ii1 + ii2 + ii3 ≤ ktaycur then
              countm12 := countm12 + 1 :
            end if:
          end do:
        end do:
      end do:
    end do:
  end do:
end do:

```

*countm12;#number of prolongations with derivatives of the total order not greater than 5*

700

(62)

```

> eqlin := Array(1 .. countm12, fill = 0) :
countm12 := 1 :
for ineq from 1 to neq do: #calculation of linearized equations
  if ineq ≤ 8 then
    ktaycur := ktay - 2 :
  else ktaycur := ktay - 3 :
  end if:
  for ii0 from 0 to ktaycur do:
    for ii1 from 0 to ktaycur do:
      for ii2 from 0 to ktaycur do:
        for ii3 from 0 to ktaycur do:
          if ii0 + ii1 + ii2 + ii3 ≤ ktaycur then
            #print("mark", ii0, ii1, ii2, ii3) :
            j := iinext[ii0, ii1, ii2, ii3] :
            #dereqcur := rtable_ref(dereq7, ineq, j) :
#dereqcur := dereq7[ineq, iinext[ii0, ii1, ii2, ii3]] :
            #print(dereq7[ineq, j]) : print(indets(dereq7[ineq, j])) :
            #print("ider", indets(dereqcur)) :
            eqlin[countm12] := coeff(evalindets(dereq7[ineq, j],
indets(dereq7[ineq, j]), vvv → linrat2(vvv)), delt, 1) :
            countm12 := countm12 + 1 :
          end if:
        end do:
      end do:
    end do:
  end do:
end do:

```

> neeq := numelems(eqlin);

neeq := 700

(63)

> nunps; nm1; nunps·nm1;

7

126

882

(64)

> ArrayDims(derivrat);

1..495, 1..11

(65)

> neq;

12

(66)

eqproc2 := proc(eq77)

*#multiplying an equation by an integer to get integer, rather than rational, coefficients*

res := Array(1 .. nm1 · nunps, fill = 0) :

lc := 1 :

for ndr from 1 to nm1 do:

for unnun from 1 to nunps do:

p3 := coeff(eq77, divlin9[ndr, unnun]) :

#print(p3, ndr, unnun) :

res[ndr + (unnun - 1) · nm1] := p3 :

if p3 ≠ 0 then lc := lcm(lc, denom(p3)) :

end if:



```

    end do:
  end do:
  lc·res:
end proc:
Warning, `res` is implicitly declared local to procedure
`eqproc2`
Warning, `lc` is implicitly declared local to procedure `eqproc2`
Warning, `ndr` is implicitly declared local to procedure
`eqproc2`
Warning, `unnun` is implicitly declared local to procedure
`eqproc2`
Warning, `p3` is implicitly declared local to procedure `eqproc2`

```

```

> eqint := eqproc2(eqlin[1]);

```

|            |                                                                                                                                                                                                                       |      |
|------------|-----------------------------------------------------------------------------------------------------------------------------------------------------------------------------------------------------------------------|------|
| $eqint :=$ | <div style="border-left: 1px solid black; border-right: 1px solid black; padding: 0 10px; display: inline-block;"> 1 .. 882 Array<br/> Data Type: anything<br/> Storage: rectangular<br/> Order: Fortran_order </div> | (67) |
|------------|-----------------------------------------------------------------------------------------------------------------------------------------------------------------------------------------------------------------------|------|

```

matgen := Matrix(neeq, nm1·nunps) :
for iilin from 1 to neeq do#calculating the matrix of coefficients
  est := eqlin[iilin]:
  matgen[iilin,..] := eqproc2(est) :
end do:

```

```

nm1·nunps;
neeq;

```

|     |      |
|-----|------|
| 882 |      |
| 700 | (68) |

```

> LinearAlgebra[Rank](matgen);

```

|     |      |
|-----|------|
| 669 | (69) |
|-----|------|

```

matgenm1 := LinearAlgebra:-DeleteColumn(matgen, 1 + 6·nm1) :
#matrix with a column for ps1r coefficients deleted

```

```

> st44 := time( ) :
LinearAlgebra[Rank](matgenm1);
time( ) - st44;

```

|        |      |
|--------|------|
| 668    |      |
| 33.437 | (70) |

```

>
> st47 := time( ) :
for inp from 1 to nunps do:
  matgenm1 := LinearAlgebra:-DeleteColumn(matgen, 1 + (inp - 1)·nm1) :
  #matrices with columns of coef for spinor components deleted
  print(inp, LinearAlgebra[Rank](matgenm1)) :
end do:
time( ) - st47;

```

|        |  |
|--------|--|
| 1, 668 |  |
| 2, 668 |  |

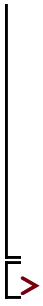

3, 668  
4, 668  
5, 668  
6, 668  
7, 668  
243.312

**(71)**
